# Supplementary material for: Promptable Game Models: Text-Guided Game Simulation via Masked Diffusion Models
Source: arXiv:2303.13472 source file (2024-01-21)
Supplement: Supplementary file 1 [file diffusion_overview.tex]

\subsection{DDPM background}
\steph{to adapt}

\footnote{In this work we model the distribution of sequences of states $\vecsequence$ and we adopt the $\vecdiffdata$ notation in this overview section to remain consistent with the diffusion model literature.} by means of latent variables in the form $p_\theta(\vecdiffdata_0) := \int p_\theta(\vecdiffdata_{0:\numdifftimesteps})dx_{1:\numdifftimesteps}$, where the latent variables $\vecdiffdata_{1:\numdifftimesteps}$ have the same dimensionality as $\vecdiffdata_0$. Several diffusion model formulations have been proposed [] and in this work we follow the DDPM formulation of [Cite Ho]. The posterior distribution over the latent variables is defined through a \emph{forward process} that consists in a fixed Markov chain with gaussian transitions in the form
\begin{equation}
q(\vecdiffdata_\difftimestep|\vecdiffdata_{\difftimestep-1}) := \mathcal{N}(\vecdiffdata_\difftimestep;\sqrt{1-\vecdiffbeta_\difftimestep}\vecdiffdata_{\difftimestep-1}, \vecdiffbeta_\difftimestep I),
\end{equation}
which can be seen as a process that gradually adds gaussian noise to the data point $\vecdiffdata_0$ following a variance schedule $\vecdiffbeta_1,...,\vecdiffbeta_{\numdifftimesteps}$.

A \emph{reverse process} maps samples from a normal distribution $p(\vecdiffdata_{\numdifftimesteps})=\mathcal{N}(\vecdiffdata_{\numdifftimesteps};0,I)$ to the approximated data distribution $p_\theta(\vecdiffdata_0)$ and takes the form of a Markov chain with learnable gaussian transitions
\begin{equation}
p(\vecdiffdata_{\difftimestep-1}|\vecdiffdata_{\difftimestep}) := \mathcal{N}(\vecdiffdata_{\difftimestep-1};\mu_\theta(\vecdiffdata_\difftimestep,\difftimestep),\sigma_\difftimestep I),
\end{equation}
where $\sigma_\difftimestep$ is fixed and depends only on the variance schedule. This process can be interpreted as gradual denoising of a noisy data sample.

To model the reverse process, we parametrize it using a neural network. Rather than directly modeling $\mu_\theta(\vecdiffdata_\difftimestep,\difftimestep)$, we adopt the $\epsilon$ parameterization of [] that predicts the applied noise instead. The denoised sample can be recovered from $\epsilon$ as $\mu_\theta(\vecdiffdata_\difftimestep,\difftimestep)=\frac{1}{\sqrt{\vecdiffalpha_{\difftimestep}}}(\vecdiffdata_\difftimestep - \frac{\vecdiffbeta_\difftimestep}{\sqrt{1 - \bar{\vecdiffalpha}_\difftimestep}}\epsilon_\theta(\vecdiffdata_\difftimestep,\difftimestep))$, where $\vecdiffalpha_\difftimestep= \sqrt{1 - \vecdiffbeta_\difftimestep}$ and $\bar{\vecdiffalpha}_\difftimestep = \prod_{i=1}^{\difftimestep}\vecdiffalpha_i$.

To train the model, we uniformly sample a diffusion timestep $\difftimestep$ and produce a noisy sample
\begin{equation}
\label{eq:diffusion_forward_sampling}
\vecdiffdata_\difftimestep := q(\vecdiffdata_\difftimestep|\vecdiffdata_0) = \sqrt{\bar{\vecdiffalpha}_\difftimestep} \vecdiffdata_0 + \epsilon \sqrt{1 - \bar{\vecdiffalpha}_\difftimestep}, \epsilon \sim \mathcal{N}(0,I).
\end{equation}
The training objective is expressed as the minimization of:
\begin{equation}
\label{eq:diffusion_loss}
\mathbb{E}_{\difftimestep,\vecdiffdata_\difftimestep \sim q(\vecdiffdata_\difftimestep|\vecdiffdata_0),\epsilon \sim \mathcal{N}(0,I)}||\epsilon - \epsilon_\theta(\vecdiffdata_\difftimestep,\difftimestep)||.
\end{equation}

Once the model is trained, sampling from the approximated data distribution $p_\theta(\vecdiffdata_0)$ can be performed by sampling $\vecdiffdata_{\numdifftimesteps}\sim\mathcal{N}(0,I)$ and following the reverse process $p(\vecdiffdata_{\difftimestep-1}|\vecdiffdata_{\difftimestep})$ to gradually denoise the sample. Please refer to [] for further details.

Diffusion models can easily be extended to support conditional data distributions $\vecdiffdata_0 \sim q(\vecdiffdata_0|c)$ by adding the conditioning information $c$ as an additional input to the model $\epsilon_\theta$.
